# Supplementary material for: MetaV: A Meta-Verifier Approach to Task-Agnostic Model Fingerprinting
Source: arXiv:2201.07391 source file (2022-05-19)
Supplement: Supplementary file 1 [file supp.tex]

\relax
%File: formatting-instructions-latex-2022.tex
%release 2022.1
\documentclass[letterpaper]{article} % DO NOT CHANGE THIS
\usepackage{aaai22}  % DO NOT CHANGE THIS
\usepackage{times}  % DO NOT CHANGE THIS
\usepackage{helvet}  % DO NOT CHANGE THIS
\usepackage{courier}  % DO NOT CHANGE THIS
\usepackage[hyphens]{url}  % DO NOT CHANGE THIS
\usepackage{graphicx} % DO NOT CHANGE THIS
\urlstyle{rm} % DO NOT CHANGE THIS
  % DO NOT CHANGE THIS
\usepackage{natbib}  % DO NOT CHANGE THIS AND DO NOT ADD ANY OPTIONS TO IT
\usepackage{caption} % DO NOT CHANGE THIS AND DO NOT ADD ANY OPTIONS TO IT
\DeclareCaptionStyle{ruled}{labelfont=normalfont,labelsep=colon,strut=off} % DO NOT CHANGE THIS
\frenchspacing  % DO NOT CHANGE THIS
\setlength{\pdfpagewidth}{8.5in}  % DO NOT CHANGE THIS
\setlength{\pdfpageheight}{11in}  % DO NOT CHANGE THIS
%
% These are recommended to typeset algorithms but not required. See the subsubsection on algorithms. Remove them if you don't have algorithms in your paper.
\usepackage{algorithm}
\usepackage{algpseudocode}
\usepackage{amsmath}
\usepackage{amssymb}
\usepackage{amsfonts}
\usepackage{booktabs}
\usepackage{makecell}

%
% These are are recommended to typeset listings but not required. See the subsubsection on listing. Remove this block if you don't have listings in your paper.
\usepackage{newfloat}
\usepackage{listings}
\lstset{%
	basicstyle={\footnotesize\ttfamily},% footnotesize acceptable for monospace
	numbers=left,numberstyle=\footnotesize,xleftmargin=2em,% show line numbers, remove this entire line if you don't want the numbers.
	aboveskip=0pt,belowskip=0pt,%
	showstringspaces=false,tabsize=2,breaklines=true}
\floatstyle{ruled}
\newfloat{listing}{tb}{lst}{}
\floatname{listing}{Listing}
%
%\nocopyright
%
% PDF Info Is REQUIRED.
% For /Title, write your title in Mixed Case.
% Don't use accents or commands. Retain the parentheses.
% For /Author, add all authors within the parentheses,
% separated by commas. No accents, special characters
% or commands are allowed.
% Keep the /TemplateVersion tag as is
% \pdfinfo{
% /Title (AAAI Press Formatting Instructions for Authors Using LaTeX -- A Guide)
% /Author (AAAI Press Staff, Pater Patel Schneider, Sunil Issar, J. Scott Penberthy, George Ferguson, Hans Guesgen, Francisco Cruz, Marc Pujol-Gonzalez)
% /TemplateVersion (2022.1)
% }

% DISALLOWED PACKAGES
% \usepackage{authblk} -- This package is specifically forbidden
% \usepackage{balance} -- This package is specifically forbidden
% \usepackage{color (if used in text)
% \usepackage{CJK} -- This package is specifically forbidden
% \usepackage{float} -- This package is specifically forbidden
% \usepackage{flushend} -- This package is specifically forbidden
% \usepackage{fontenc} -- This package is specifically forbidden
% \usepackage{fullpage} -- This package is specifically forbidden
% \usepackage{geometry} -- This package is specifically forbidden
% \usepackage{grffile} -- This package is specifically forbidden

% \usepackage{hyperref} % -- This package is specifically forbidden
% \hypersetup{
%     colorlinks=true, %set true if you want colored links
%     linktoc=all,     %set to all if you want both sections and subsections linked
%     citecolor=blue,
%     linkcolor=blue,  %choose some color if you want links to stand out
% }

\usepackage{enumitem}
\setlist[itemize]{leftmargin=*}
\setlist[enumerate]{leftmargin=*}
\usepackage{multicol}
\usepackage{multirow}

\setcounter{secnumdepth}{2} %May be changed to 1 or 2 if section numbers are desired.

% The file aaai22.sty is the style file for AAAI Press
% proceedings, working notes, and technical reports.
%

% Title

\usepackage{xcolor}

% Your title must be in mixed case, not sentence case.
% That means all verbs (including short verbs like be, is, using,and go),
% nouns, adverbs, adjectives should be capitalized, including both words in hyphenated terms, while
% articles, conjunctions, and prepositions are lower case unless theyapproach
% directly follow a colon or long dash
\title{Technical Appendix for \\ 
UTAF: A Universal Approach to Task-Agnostic Model Fingerprinting}
\author{
    %Authors
    % All authors must be in the same font size and format.
    Anonymous Author(s)
}
% \affiliations{
% Submission \# 6768
% }

\begin{document}

\maketitle

%%%%%% ABSTRACT
\appendix
\input{tex/app.tex}

%%%%% OTHER PARTS

\newpage
% argument is your BibTeX string definitions and bibliography database(s)
\bibliography{ref}

\end{document}
